# Supplementary material for: An Improved Reinforcement Learning Algorithm for Learning to Branch
Source: arXiv:2201.06213 source file (2022-01-17)
Supplement: Supplementary file 1 [file appendix.tex]

\section*{Appendix}

Here are the parameters used for our proposed algorithm.

% \begin{table*}[h]
%     \centering
%     \begin{tabular}{cc}
%          \hline
%          Name & Used value\\
%          \hline
%          Optimizer & \textit{Adam}\\
%          Batch size & 32 for \textit{Balanced Item Placement} and \textit{Anonymous Problem}\\
%             & 24 for \textit{Workload Apportionment}\\
%          Learning rate & 0.001\\
%          $ \varepsilon $-greedy policy & $ \varepsilon = 0.01 $~\cite{van2016deep}\\
%          Dimension of input embedding in GCNN & 64\\
%          Replay buffer size & 100K for \textit{Balanced Item Placement} and \textit{Anonymous Problem}\\
%             & 20K for \textit{Workload Apportionment}\\
%          Discount factor & 0.99\\
%          Period for target model's hard update & 500\\
%          Period for evaluating the trained policy & 1000\\
%          Epochs & 50K\\
%          \hline
%     \end{tabular}
%     \caption{Hyperparameters setting}
%     \label{tab:my_label}
% \end{table*}

\begin{itemize}
    \item Optimizer: Adam
    \item Batch size: 32 for \textit{Balanced Item Placement} and \textit{Anonymous Problem}, 24 for \textit{Workload Apportionment}
    \item Learning rate: 0.001
    \item $ \varepsilon $-greedy with $ \varepsilon = 0.01 $, same used by Double DQN~\cite{van2016deep}
    \item Dimension of input embedding in GCNN: 64
    \item Replay buffer size: 100K for \textit{Balanced Item Placement} and \textit{Anonymous Problem}, 20K for \textit{Workload Apportionment}
    \item Discount factor: 0.99
    \item Period for target model's hard update: $ \tau^t $ = 500
    \item Period for evaluating the trained policy: $ \tau^s $ = 1000
    \item Epochs: 50K
\end{itemize}
